# Supplementary material for: HPFF: Hierarchical Locally Supervised Learning with Patch Feature Fusion
Source: arXiv:2407.05638 source file (2024-07-09)
Supplement: Supplementary file 1 [file X_suppl.tex]

\clearpage
\setcounter{page}{1}

\section{Datasets}
In this section, we provide a brief introduction to the four image classification datasets that we utilized, as well as the data augmentation methods employed.

SVHN {\cite{netzer2011reading}} is a real-world image dataset used for developing machine learning and object recognition algorithms, especially for recognizing digits in visual objects. 
It is derived from Google Street View data and contains over 600,000 images of digits, covering 10 classes (0-9). Each image is a 32$\times$32 pixel color image.

CIFAR-10 {\cite{krizhevsky2009learning}} dataset contains 60,000, 32$\times$32 color images, divided into 10 classes, with 6,000 images per class. 
These classes include airplanes, cars, birds, cats, deer, dogs, frogs, horses, ships, and trucks. The dataset is divided into 50,000 training images and 10,000 test images.

STL-10 {\cite{coates2011analysis}} dataset is designed to evaluate unsupervised feature learning and self-learning algorithms. 
It is inspired by the CIFAR-10 dataset but has some changes. 
It includes 10 classes, each with 500 training images and 800 test images. 
All images are 96$\times$96 color images. 
In addition, an unlabeled dataset is provided, containing 100,000 additional images.

ImageNet {\cite{deng2009imagenet}} is a large-scale visual database composed of over 10 million high-resolution images with detailed labels. 
These images cover more than 20,000 categories, with the number of images per category ranging from a few hundred to tens of thousands. 
The goal of ImageNet is to provide researchers with an easily accessible, large-scale image database to assist them in their research in computer vision and other fields.

\section{Generalization Study}
In this section, we study the generalization of our proposed HiLo. We directly use the checkpoints trained on the CIFAR-10 \cite{krizhevsky2009learning} dataset for testing on the STL-10 \cite{coates2011analysis} dataset, which is inspired by \cite{60}. 

From Table \ref{Table 1}, we can observe a significant difference in the generalization abilities between DGL and BP. However, after adding our HiLo method, the test accuracy improved significantly, even surpassing BP. Based on these results, we can infer that HiLo, by facilitating information interaction between local modules, enhances the generalization ablity of supervised local learning method.

\begin{table}[htbp]
	\centering

 \scalebox{0.95}{
	\begin{tabular}{ccc}\hline
Method&ResNet-32 (K=16)&ResNet-110 (K=55)\\ \hline
BP & 35.98 & 36.78 \\
DGL \cite{belilovsky2019greedy} & 31.95 & 33.16 \\
\bfseries{DGL*} & {\bfseries 39.06} & {\bfseries 40.62}\\ \hline
	\end{tabular}}
 \caption{Generalization study. Checkpoints are trained on the CIFAR-10 dataset and tested on the STL-10 dataset. The data in the table represents the test accuracy.}
     \label{Table 1}
\end{table}
